# Supplementary material for: Prediction of Performance and Power Consumption of GPGPU Applications
Source: arXiv:2305.01886 source file (2023-05-03)
Supplement: Supplementary file 1 [file AppC.tex]

\chapter{Appendix C} % Main appendix title

\label{AppendixC}

\section{Appendix C. \emph{Author's Response to Reviewers Comments}}

\begin{flushright}\text{RC: Reviewer's Comment, AR: Author's Response}
\end{flushright}
\begin{flushleft}
\large{Dear Reviewers}
\end{flushleft}
\large{ We would like to thank the reviewers for providing valuable comments on the thesis. The comments are helpful and constructive for improving the quality of the thesis.
Thank you for your valuable feedback. We address the concerns raised by you below. }

\section{Reviewer \#1}

\subsection{Chapter 1}
\subsubsection{Comment \#1}
\textbf{RC: What is the logic of adding both performance and power consumption in one thesis? The link between power consumption and performance is not very clear. The author should explain the reasoning of combining both in one thesis and also explain how one affects the other, i.e., how power affects the performance} \\
AR:   
As mentioned in Chapter \ref{ch:introduction}, the objective of the thesis is to investigate static-analysis based energy prediction modeling of CUDA applications. Since energy consumption is a product of power consumption over the GPU's execution time, it becomes necessary to investigate power consumption and performance modeling. Many past studies on GPU have combined the two considering their impact on energy consumption\cite{Abe2012,Jiao2010,Hong2010,Wang2014PerformanceAP}. We already explained this rationale in our thesis. 

Although power and performance do not have a one-to-one relationship, if an application performs poorly, it will lead to inefficient use of power. Also, it is observed that common program and architecture features affect both performance and power consumption of GPU \cite{Hong2010,Abe2012}. A recent study~\cite{coplin2015effects} also demonstrates that fine-tuning a GPGPU program only for performance hurts power consumption. 
We are aware that the investigation of the intricate relationship between power consumption and performance is a new research topic in itself.

{\em Our objective through this work is not to understand how performance affects power or vice versa but to measure the performance and power of GPU applications to predict their energy consumption}.  We want to investigate the relationship between the application's performance and power consumption as an extension of this body of research in the future. This may include studying the trade-off between the increase in power or performance and its impact on each other.      

\subsubsection{Comment \#2 Comment \#9}
\textbf{RC: Why not use machine learning for predicting the execution time also? What is the advantage of predicting power consumption using machine learning versus 
other non-machine learning approaches? Please include a discussion on this.
} \\
AR: Both analytical and machine learning models are valuable tools in data-driven analysis. Analytical models are based on mathematical equations and statistical methods and can provide a causal explanation. Hence, analytical models are utilized when the underlying relationships between variables are well understood. Machine learning algorithms, on the other hand, can capture more complex and non-linear relationships between variables. Machine learning models can learn from large amounts of data and identify patterns that may not be apparent through analytical methods. %In summary, the choice between using an analytical model or a machine learning model will depend on the specific problem, the quality and quantity of available data, and the level of complexity of the relationships between variables. 

Analytical models have been implemented for performance prediction of GPUs in the past \cite{Hong2009, Kothapalli2009, Baghsorkhi2010}. Amaris et al. \cite{Amaris2016} compared the results of analytical and machine learning models and concluded that analytical models are more precise than the other machine learning approach. Our approach of using an analytical model to predict execution time can be {\em extended to build an assistance-type tool to highlight the execution bottlenecks beyond just execution time}. We could have used Machine Learning for execution time as well. However, since our larger goal is to provide design assistance, it remains to be seen how an ML model can provide a clear, reliable, and concise explanation like an analytical model. 

Factors that influence the power consumption of a GPU have a complex non-linear relationship among its operating components. We have demonstrated this in Chapter \ref{ch:powerpred}. A data-driven power prediction model is an alternate approach that can deal with this non-linearity to estimate power consumption. 

Due to the inherent generality in the data-driven approach, a data-driven model with sufficient data points has the potential to capture the complexity arising out of the diversity of different components of a GPU acting together to execute a code. Of course, the model must be adequately trained with a large size and diversity of the dataset used for learning. The generality of a data-driven approach lies in the fact the model does not require any functional properties or physical characteristics of the components inside a GPU, nor does it require any minute architectural details of a GPU. Thus, modeling power consumption using an ML makes practical sense. Moreover, in our approach, we have consciously tried to increase the diversity by choosing benchmarks with different characteristics, which could be a reason for the robustness of the model demonstrated in the thesis. 

The relationship between GPU characteristics and power consumption by a CUDA application, which can be reasonably captured from a data-driven approach, becomes hard to model using an analytical approach. The scheduling algorithm defined in Chapter~\ref{ch:execTime} estimates the cycle time for each instruction, which can be used to determine the total execution time; however, such an approach won’t work to estimate the power consumed by each instruction. The main reason is that the computation of power consumption at the instruction level is not feasible or reasonably accurate. Hence, the same analytical approach to scheduling instructions will not work for a static analysis-based power prediction approach. On the other hand, ML models have been able to learn latent relationships that influence power consumption (from a data set), which are not possible to capture through analytical methods.  

Another objective of our research is to ensure a reasonable amount of generality in our solution. Our analytical model for execution time prediction and the data-driven approach for power prediction is sufficiently generalizable. 

In Chapter \ref{sec:whymlforPower}, we discussed why we could not build an analytical model for power prediction.
\subsection{Chapter 4}

\subsubsection{Comment \#3}
\textbf{RC: Algorithm 5: what are the input and output? Need to mention this. } \\
AR:  We have now explicitly added input and output for Algorithms \ref{delay_algorithm} and \ref{simulation}.

\subsubsection{Comment \#4}
\textbf{RC: Why do you need a scheduling algorithm to predict the execution time?
}\\
AR: Analytical models are built to capture interactions between software and hardware for execution time prediction. To improve the accuracy of the analytical model,  we used a scheduling algorithm with which the model can achieve instruction-level granularity by mapping the instructions to the allocated resource. This, in turn, can estimate the execution time of an instruction, and the total execution time. This has been explained in Chapter \ref{ch:execTime}. Prior research has also acknowledged that a scheduling algorithm helps to build an accurate prediction model \cite{Kothapalli2009, resios2011, amaris2015} of a GPU.

\subsubsection{Comment \#5}
\textbf{RC: For figure 4.3, there is no explanation on the quality of the result – how close are the predicted values to the actual values for execution time?
}\\
AR: As mentioned in Chapter 4, we have presented two models. We found shortcomings of the first model (Chapter 4.4) and moved on to build an improved model presented in Chapter \ref{PP_approach2}. Instead of providing only the improved model, we included both models to maintain the chronology and provide the holistic journey of arriving at a better model from our first attempt. As we have built a better model, we did not present the results of the first model in detail. However, based on the comment, we have now added the results of the first model for each benchmark in Table \ref{gpu_model1}.

\subsubsection{Comment \#6}
\textbf{RC: The mean absolute error values given in table 4.2 seem to be high? What is the reason for this?  
}\\
AR:  Performance prediction is difficult, especially for parallel computers such as GPUs, considering its complex architecture and different types of memory hierarchy \cite{Kothapalli2009, Konstantinidis2017AQR, Hong2010, resios2011, volkov2016}. The error in prediction could be due to missing runtime information such as branch divergence, cache behavior, runtime occupancy, access patterns, bank conflicts etc.  

Considering this fact, in comparison to existing studies (Table \ref{tab:existing approaches}), the observed results are decent and acceptable for a completely static-analysis based model. Performance prediction results, if reasonable, can be used as a guiding tool for performance prediction rather than taking the predicted value as an absolute truth. Reviewers of our CPE Journal publication acknowledged the fact that performance prediction is hard and observed results are decent.

We have added a Table \ref{tab:existing approaches} for presenting the comparative study of results for existing performance prediction studies versus our approach. 

\subsubsection{Comment \#7}
\textbf{RC: The author should include a Section discussing the limitations of the given study
}\\
AR: We have included Chapter \ref{limitations_approach1} which discusses the limitations of the proposed model. 

\subsection{Chapter 5}

\subsubsection{Comment \#8}
\textbf{RC: In chapter 5 on ML-based power prediction, does the learning happen statically, or can the system becomes better at prediction by continuously learning at run-time, as more data is fed to it? In other words, is the proposed prediction model adaptive? This would be a useful feature
to have in the real world.
}\\
AR: We have not included any discussion on adaptive learning models in the thesis since these continuous learning approaches will need runtime data. Our goal through this work was to predict power using static and one-time dynamic analysis. We are investigating the feasibility of using adaptive learning methods for power prediction as part of future work. 

\section{Reviewer \#2}

\subsection{Chapter 4}
\subsubsection{Comment \#1}
\textbf{RC: The parameter sz\_m will depend on the actual memory global/shared/etc. May be better to
qualify the parameter accordingly.}\\
AR:  We have now separated $sz\_m$  to Sz\_{gm} for global memory, and Sz\_{sm} for shared memory. This will help for better readability. 

\subsubsection{Comment \#2}
\textbf{RC: The value of 47 cycles for shared memory access is not always accurate since the actual number can vary based on the number of bank conflicts per access. Did this result in some
inaccuracy in the predicted performance?}\\
AR:  The result of 47 cycles for shared memory access result did not add inaccuracy in the predicted performance since we have used a shared memory penalty in our model which is based on runtime data. This dynamic model helps to model the runtime behaviour of shared memory due to bank conflicts. 

\subsubsection{Comment \#3}
\textbf{RC: 4.3: Results: Is there a comparison of the accuracy across the papers that do GPU
performance modeling? The errors reported in Table 4.2 are beyond 25\% in most cases. The
utility of the proposed model vis-a-vis existing models is therefore useful.}

AR: We have added a Table \ref{tab:existing approaches} for presenting the comparative study.  As seen in the table considering the size of the dataset used for testing and the variation in benchmark characteristics, our model shows decent results.

\subsubsection{Comment \#4}
\textbf{RC: 4.4.1: Isn't branch divergence serialized? This is one reason why GPU programs should not
have branch divergence. Estimating this with the longest branch time may result in
inaccuracies.}\\
AR: We agree that branch divergence is a critical issue in the performance estimation of GPU programs. However, as already mentioned in the limitation of the performance model, predicting branch behaviour statically for all types of scenarios in different applications is a hard problem. Work by Sarkar et al. \cite{sarkar2015profile} also reinforces the fact that predicting divergence is impossible using purely static analysis based approach. One needs to run the program multiple times to capture the pattern of branch divergence. We would like to study it in the future if this behavior can be modeled using runtime data. It was already included in Chapter \ref{ch:conclusion} as future work.

\subsubsection{Comment \#5}
\textbf{RC : 4.4.2.2: The relation between SMs and blocks is complicated. It is based on available
resources and how many blocks can be scheduled based on the available resources. There are
some upper limits, but usually more blocks per SM are assigned if there are enough resources
on the SM.}\\
AR: We understand that the accurate runtime behaviour of allocation of blocks to SMs is hard to predict.  However, considering the assignment is based on resource allocation, we have considered both factors for the allocation of blocks to SMs in model proposed in Chapter 4.4 :
\begin{itemize}
    \item the availability of number of active blocks (hardware limit) 
    \item resource allocation for active blocks 
\end{itemize}

\subsubsection{Comment \#6}
\textbf{RC :4.4.3: Did the work consider rare occasions when the application program uses explicit
synchronization primitives? These forced synchronization operations that act across a warp
or across a block have a huge impact on the ability of analytical methods to predict the run
time.}\\
AR:  Although considering the impact usage of explicit synchronization primitives in a program is a very crucial problem. We have not considered the impact of synchronization primitives since predicting it statically is a hard problem. Since this problem cannot be addressed statically, we plan to study this as a future work using runtime data. We have included this as a future work in Chapter \ref{ch:conclusion}.

\subsubsection{Comment \#7}
\textbf{RC: From Figure 4.8, 4.11: we do notice an average error of close to 12\%, and the error varies
across applications. What could be the reasons for this behavior? Is this completely explained in
4.4.11?}\\
AR: We have mentioned in the results that considering the fact that the benchmarks under study belong to different types of communication and computation patterns (compute or memory bound), size of occupancy, and access patterns, the observed error will vary across applications. Considering the constraints of static analysis-based models, the model behavior of these application features is hard, resulting in the observed error.   

\subsection{Chapter 5}

\subsubsection{Comment \#8}
\textbf{RC:  From Figure 5.11, there is very little difference in performance across the methods. Figure 5.11 can include the min/max difference between the actual power usage and the predicted power usage as a percentage. } \\ 
AR:  Considering the number of data points in the plot, we did not modify Figure 5.11. Instead, we have now included a Figure \ref{fig_errorinpredict} for presenting the prediction error for better readability and clarity.

\subsubsection{Comment \#9}
\textbf{RC: Chapters 4 and 5 deal with predicting time and power
consumption. It will be good to compare and see if the tough instances from Chapter 4
correspond to the tough instances in Chapter 5. Are the factors that adversely impact the
prediction of run time also impacting the prediction of power consumption? How are rare
features such as synchronization addressed in the power prediction model? What are the
assumptions for the model designed in Chapter 5?}\\ 
AR: We have now compared the high error results for execution time with their power prediction results. We have chosen 20 benchmarks whose execution time prediction error is greater than 15\%. We have presented the comparison for these results in Figure \ref{Fig:exectimepower}. As seen in the plot, apart from the Convolution Separable benchmark, errors for all other benchmarks are not consistent for execution time and power. When we analyzed the Convolution Separable benchmark in detail to understand why both the models fail to predict, we observed that the difference between instructions issued (18420093) and instructions executed (11943936) for this benchmark is quite high for {\tt convolutionRowsKernel}. This could be due to hardware-level optimizations which our model failed to predict. The power prediction model seems to perform better in comparison with execution time prediction.

Synchronization is counted as a miscellaneous instruction, and its impact is observed through feature contribution. 

We have added the assumptions for the power prediction model in Chapter \ref{power_assumptions}. 

\subsection{Chapter 6}

\subsubsection{Comment \#10}
\textbf{RC: Usually, it is likely that the prediction accuracy depends on the input size also. So, how is this
input provided in the tool? How is the input size impacting the models from Chapters 4 and 5?
Are the parameters obtained via microbenchmarks integrated with the tool? } \\
AR:   We have considered input size and its effect on resource usage by taking the launch parameters (grid size, block size ) of the CUDA kernel as user input. We also take a number of loop iterations for loops present in the kernel. Program Feature Extraction Algorithm (PFEA) presented in the paper schedules instructions on GPU based on these inputs, which are mapped to the GPU hardware resources based on resource constraints.  

We have elaborated on the influence of input size on resource usage in Chapter \ref{ch:execTime}. To summarize-- in order to estimate resource usage through static analysis, we create a flat trace of the control-flow graph of the program. The Mergesort program has a for-loop, whose iteration count is dependent on the input size. We flatten the loop by multiplying the instruction set, which constitutes the loop body, by the loop count. For instance, if the loop body has two {\tt add} instructions and the loop count is 3, then we create 6 add instructions. 
Next, we schedule these instructions on the hardware resources based on the hardware specifications provided by the vendor. This scheduler, in a sense, models the impact of input size on resource usage. 

We have tested that the results of models from Chapters \ref{ch:execTime} and \ref{ch:powerpred} are able to predict the execution time with the change in input. 

The microbenchmarks are incorporated into the tool and executed only once for a new architecture. Microbenchmarks are part of the setup phase for the prediction tool. During setup, the microbenchmarks are automatically executed, and the results are stored in the application for the underlying architecture. Results generated using microbenchmarks are then utilized in predicting execution time and power. 

\subsubsection{Comment \#11}
\textbf{RC:
Newer generations of CUDA hardware have introduced additional architectural and programming
features such as tensor cores, multi-kernel execution, special instructions, and the like. The
impact of these on the models may be indicated \\ }
AR: We are aware of these new features introduced in the new architecture and we did not investigate the impact of these major architectural changes in our thesis. We have mentioned this in Chapter \ref{ch:conclusion} in the thesis.
